# Supplementary material for: Self-Improvement in Language Models: The Sharpening Mechanism
Source: arXiv:2412.01951 source file (2024-12-04)
Supplement: Supplementary file 1 [file appendix_framework.tex]

\begin{proof}[Proof for \cref{ex:greedy}]
  
\end{proof}

  \begin{propmod}{prop:bestofn_inference}{$'$}[Inference-time \BestofN]
    \label{prop:bestofn_inference_general}
    Let a prompt $x\in\cX$ be given. For any $\deltafail\in(0,1)$ and
    $\gamma\in[0,1)$,
    as long as
        \begin{align}
      N \geq \frac{\log(\deltafail^{-1})}{\piref(\Ygamma(x)\mid{}x)},
        \end{align}
        inference-time \BestofN sampling produces a response
        $
    \yhat\in\Ygamma(x)$ with probability at least $1-\deltaf$.
  \end{propmod}

\begin{proof}[\pfref{prop:bestofn_inference_general}]
    Fix a prompt $x \in \cX$, failure probability $\deltaf \in (0, 1)$,
    and parameter $\gamma\in(0,1)$.
    
    By definition of the set $\Ygamma(x)$, $\yhat \in \Ygamma(x)$ if
    and only if there exists $i \in [N]$ such that $y_i\in\Ygamma(x)$. The complement of this event, i.e., that $y_i \notin \Ygamma(x)$ for all $i \in [N]$, has probability 
    \begin{align}
        \Pr\prn*{y_i \notin \Ygamma(x),{}\forall i \in [N]} = \prn*{1 - \piref(\Ygamma(x)\mid{}x)}^N.
    \end{align}
    Rearranging the \rhs, we have 
    \begin{align}
        \prn*{1 - \piref(\Ygamma\mid{}x)}^N 
        =&~ 
        \exp\prn*{-N\log\prn*{\frac{1}{1-\piref(\Ygamma\mid{}x)}}}
        \le
        \exp\prn*{-N\cdot\piref(\Ygamma\mid{}x)},
    \end{align}
    since $\log(x) \ge 1-\frac{1}{x}$ for $x > 0$, which implies that $\log\prn*{\frac{1}{1-\piref(\Ygamma\mid{}x)}} \ge \piref(\Ygamma\mid{}x)$. 
    Thus, as long as $N \ge
    \frac{\log(\deltaf^{-1})}{\piref(\Ygamma\mid{}x)}$, we have
    \begin{align}
        \Pr\prn*{y_i \notin \Ygamma(x),{}\forall i \in [N]} 
        \le 
        \exp\prn*{-N\cdot\piref(\Ygamma\mid{}x)}
        \le 
        \exp(-\log(\deltaf^{-1})) = \deltaf. 
    \end{align}
    We conclude that with probability at least $1-\deltaf$, there exists $i \in [N]$ such that $y_i \in \Ygamma(x)$, and $\yhat \in \Ygamma(x)$ as a result.  

\end{proof}
